# Supplementary material for: Discovery and Contextual Data Cleaning with Ontology Functional Dependencies
Source: arXiv:2105.08105 source file (2022-03-13)
Supplement: Supplementary file 1 [file appendix.tex]

\blue{\section{Appendix} \label{sec:appendix}
\subsection{Proof of Theorem 12}
We first proof (1) each $\tau$-constrained repair is a minimal repair. Assume $(I', S')$ is a $\tau$-constrained repair, based on definition in Section~\ref{sec:reptype1}, there is no repair $(I'', S'')$ for all the senses such that $dist(S, S'')$ is smaller than $dist(S, S')$ and $dist(I, I'')$ is smaller than $\tau$. Since $dist(I, I') \leq \tau$, there is no other repair $(I'', S'')$ for all the senses such that $dist(S, S'')$ is smaller than $dist(S, S')$ and $dist(I, I'')$ is smaller than $dist(I, I')$. In other word, $(I', S')$ is a minimal repair.
}

\blue{
In the following, we prove (2) by contradiction. Assume that $(I', S')$ is a minimal repair but not a $\tau$-constrained repair, then there exists a repair $(I'', S'')$ such that $dist(S, S'')$ is smaller than $dist(S, S')$ and $dist(I, I'')$ is smaller than $\tau$.  Repair $(I'', S'')$ is a minimal repair because no other repair can dominate $(I'', S'')$ with respect to distances to $I$ and $S$. Since $(I', S')$ is a minimal repair, then $dist(I, I'') \geq dist(I, I')$ (otherwise, $(I'', S'')$ dominates $(I', S')$). In this case, the value of $\tau$ is in the range of $[dist(I, I'), dist(I, I''))$ (otherwise, with a bound $\tau$, there are two minimal repairs), which contradicts the fact that $dist(I, I'')) \leq \tau$.}
